# Supplementary material for: Correlated Particle Motion and THz Spectral Response of Supercritical Water
Source: arXiv:2104.06888 ancillary file (2021-04-14)
Supplement: Supplementary file 1 [file si.pdf]

**Supplemental Material to**

# Correlated Particle Motion and THz Spectral Response of Supercritical Water

Maciej Śmiechowski*

*Department of Physical Chemistry, Chemical Faculty,*

*Gdańsk University of Technology, Narutowicza 11/12, 80-233 Gdańsk, Poland and*

*Lehrstuhl für Theoretische Chemie, Ruhr-Universität Bochum, 44780 Bochum, Germany*

Christoph Schran, Harald Forbert, and Dominik Marx

*Lehrstuhl für Theoretische Chemie, Ruhr-Universität Bochum, 44780 Bochum, Germany*

(Dated: December 16, 2015)

* Corresponding author. Electronic mail:

Maciej.Smiechowski@pg.gda.pl

## I. COMPUTATIONAL METHODS AND DETAILS

For our simulations we selected two state points in the supercritical regime at a temperature of $T = 660$ K, namely at $\rho = 0.2$ g/cm$^3$ (low-density supercritical water, LD–SCW) and at $\rho = 0.6$ g/cm$^3$ (high-density, HD–SCW). For comparison purposes we also performed simulations at ambient conditions, i.e. at $T = 300$ K and $\rho = 0.997$ g/cm$^3$ (room-temperature water, RTW). The standard system consisted of 128 $H_2O$ molecules in a periodic cubic box that has been resized to obtain the desired density. To test the convergence of observables, we also simulated larger systems consisting of 256 and 512 $H_2O$ molecules at the same densities, *vide infra*.

The flexible SPC water model with anharmonic stretch-stretch and stretch-bend coupling terms was used [1] as implemented in the MDynaMix software package [2] used. This water force field has been selected since it has been demonstrated previously that the flexible models of the SPC family perform particularly well in reproducing the experimental liquid-vapor coexistence curve up to and including the critical point [3]. After careful thermalization for at least 4 ns, molecular dynamics simulations in the $NVT$ ensemble were continued for 1 ns using a $\delta t = 0.25$ fs time step. The temperature was controlled by coupling to an external Nosé-Hoover thermostat. For each system, 40 to 50 $NVT$ configurations were selected to spawn 20 ps $NVE$ simulations that were used to calculate the presented spectra based on the respective time correlation functions, thus providing proper averages in the canonical ensemble.

## II. STRUCTURAL ANALYSES

### A. Hydrogen Bond Definition and Clustering Properties

In order to determine if two water molecules are hydrogen bonded (H-bonded), we follow here a variant of the common geometric criterion $R_{\mathrm{OO}} < R_{\mathrm{OO}}^{\mathrm{crit}}$ and $\beta_{\mathrm{HOO}} < \beta_{\mathrm{HOO}}^{\mathrm{crit}}$, see e.g. Ref. 4. Specifically, following earlier investigations on the H-bond definition in liquid water [5], we first construct a two-dimensional distribution function $g(R_{\mathrm{OO}}, \beta_{\mathrm{HOO}})$ in a manner analogous to radial distribution functions so that

$$g(R) = \frac{dn_{\mathrm{O}}(R)}{\rho 4\pi R^2 dR}, \tag{S1}$$

$$g(R,\beta) = \frac{dn_{\mathrm{O}}(R)}{\rho 2\pi R^2 \sin\beta dR d\beta}. \tag{S2}$$

We then define the potential of mean force (PMF),

$$W(R,\beta)/k_{\mathrm{B}}T = -\ln g(R,\beta), \tag{S3}$$

that is illustrated in Fig. S1 for the RTW system. The plot shows a pronounced basin of low PMF values that has a minimum at about $R_{\mathrm{OO}} = 2.72$ Å and $\beta_{\mathrm{HOO}} = 0°$ and features a clear saddle point at about $R_{\mathrm{OO}} = 3.20$ Å and $\beta_{\mathrm{HOO}} = 37°$. We find the delimiting contour of this basin to be adequately approximated by a simple polynomial contour (apart from small deviations at low $R_{\mathrm{OO}}$ being caused by configurations that are $> 5\,k_{\mathrm{B}}T$ above the relative free energy minimum) and we expanded here $\beta_{\mathrm{HOO}}$ in powers of $R_{\mathrm{OO}}$ up to the fourth order, obtaining the final criterion for H-bonding between the two water molecules as

$$\beta_{\mathrm{HOO}} < -3.5963\cdot 10^4 + 4.9484\cdot 10^4 R_{\mathrm{OO}} - 2.5545\cdot 10^4 R_{\mathrm{OO}}^2 + 5.867\cdot 10^3 R_{\mathrm{OO}}^3 - 5.0563\cdot 10^2 R_{\mathrm{OO}}^4, \tag{S4}$$

where $\beta_{\mathrm{HOO}}$ is measured in degrees and $R_{\mathrm{OO}}$ in Ångstrom. This definition (shown as a thick black line in Fig. S1) gives the average number of H-bonds per water molecule in RTW equal $\langle n_{\mathrm{HB}} \rangle = 3.68 \pm 0.07$, very close to the formerly obtained value of 3.60 (for a rigid-body SPC/E water model) [5]. The same criterion applies to the analyses of the two sets of SCW trajectories which has been explicitly checked.

The calculation of the extent of H-bonding in the system allows for the definition of "clusters" of water molecules as separate aggregates of molecules being topologically connected with H-bonds and separated from the rest of the system. Therefore, the cluster size satisfies

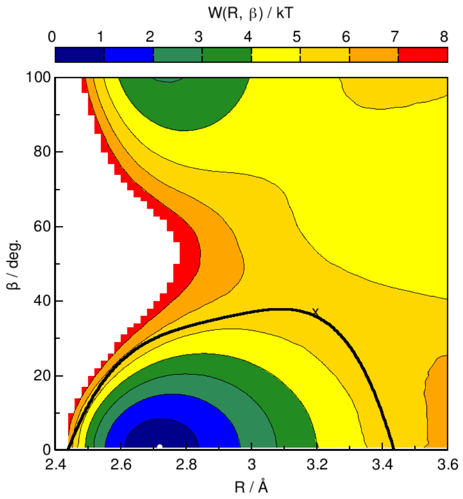


Figure S1. Two-dimensional free energy landscape or PMF, $W(R, \beta)$ according to Eq. (S3), of the RTW system plotted in units of $k_{\mathrm{B}}T$. The global minimum of the PMF is marked with a white dot and the saddle point is shown with a black cross. The thick black line denotes the criterion use to define pairs of H-bonded water molecules according to Eq. (S4).

the condition $1 \leq n_{\mathrm{c}} \leq n_{\mathrm{tot}}$ where $n_{\mathrm{tot}}$ is the system size. The average number of H-bonds per molecule and the average number of clusters for each state point considered are compiled in Table I. A detailed analysis of cluster size distribution is included in the main text (see Fig. 2 therein).

Table I. Average number of H-bonds per molecule and average number of clusters for the studied systems with 128 $H_2O$ molecules

| System | $\langle n_{\mathrm{HB}} \rangle$ | $\langle N_{\mathrm{C}} \rangle$ |
|---|---|---|
| LD–SCW | $1.00 \pm 0.12$ | $65.4 \pm 6.5$ |
| HD–SCW | $1.84 \pm 0.11$ | $19.2 \pm 5.2$ |
| RTW | $3.68 \pm 0.07$ | $1.0 \pm 0.1$ |

### B. Radial Distribution Functions

In the main text only $g_{\mathrm{OO}}(r)$ is shown explicitly in Fig. 1 to demonstrate the excellent agreement of the simulated SCW data with the available experimental data at matching densities (0.23 g/cm$^3$ [6] and 0.58 g/cm$^3$ [7]). Here we demonstrate that also the $g_{\mathrm{OH}}(r)$ and

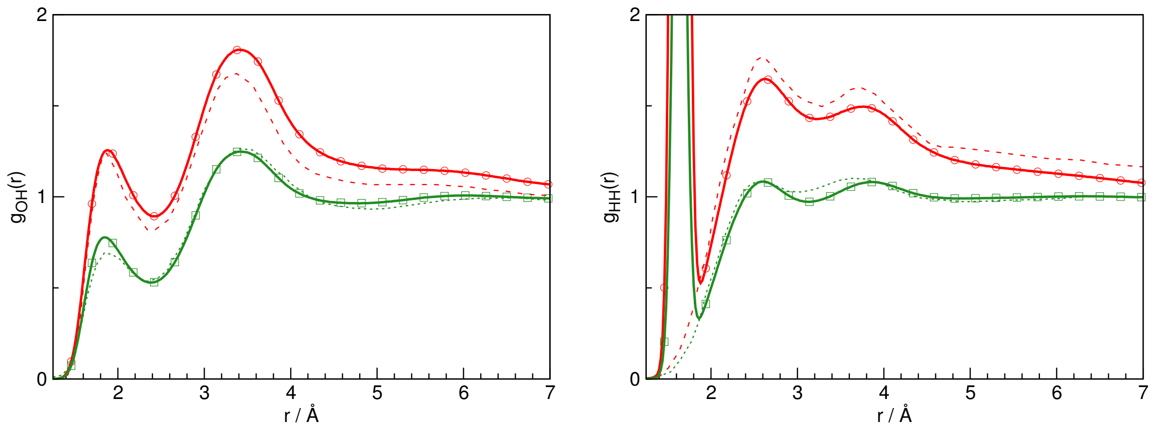


Figure S2. Radial distribution functions $g_{\mathrm{OH}}(r)$ (left) and $g_{\mathrm{HH}}(r)$ (right) for LD–SCW (red line with open circles) and HD–SCW (green line with open squares) compared to experimental data at $\rho = 0.23$ g/cm$^3$ (Ref. 6, thin dashed line) and 0.58 g/cm$^3$ (Ref. 7, thin dotted line), respectively.

$g_{\mathrm{HH}}(r)$ correlation functions compare most favorably with experiment. The relevant radial distribution functions are illustrated in Fig. S2.

### C. Convergence of Results with System Size

As mentioned above, in order to investigate the adequacy of our standard system size of 128 $H_2O$ molecules for the present purpose, we also simulated the systems using larger boxes of 256 and 512 molecules at the same respective densities. In Fig. S3, we demonstrate the convergence of the standard system size for all three partial RDFs as well as for the distribution function of the H-bond number per water molecule at both supercritical conditions studied. It is readily seen that increasing the system size has a negligible influence on the presented observables so that both the radially averaged structure and the local H-bonding pattern of each water molecule is preserved when reducing the system size. Therefore, we conclude that the system composed of 128 $H_2O$ molecules is sufficient for the present study and, in particular, for the spatial dissection of spectra.

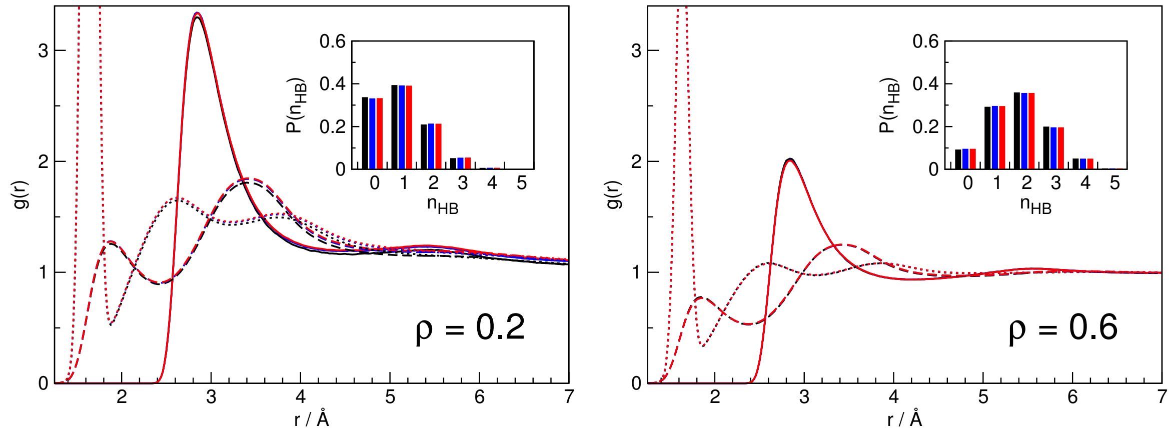


Figure S3. Radial distribution functions $g_{\mathrm{OO}}(r)$ (solid lines), $g_{\mathrm{OH}}(r)$ (dashed lines), and $g_{\mathrm{HH}}(r)$ (dotted lines) in the $N = 128$ (black), 256 (blue), and 512 (red) system at $\rho = 0.2$ g/cm$^3$ (left panel) and 0.6 g/cm$^3$ (right panel). The inset shows the distribution of the water molecules according to the number of H-bonds formed using the same color code.

## III. VIBRATIONAL DENSITY OF STATES

The usual definition of the vibrational density of states (VDOS) involves an ensemble average of the time autocorrelation funtion of mass-weighted atomic velocities, $\boldsymbol{u}_i(t) \equiv \sqrt{m_i}\boldsymbol{v}_i(t)$, over all atoms in the system, i.e.

$$I(\omega) = \int_{-\infty}^{\infty} dt\, \mathrm{e}^{-i\omega t} \;\; \langle \boldsymbol{u}_i(0)\boldsymbol{u}_i(t)\rangle \ , \tag{S5}$$

which are thus treated independently. In the case of water, this offers the possibility to separate in a straightforward manner the individual contributions stemming from O and H single-particle dynamics by ensemble averaging over the relevant class of atoms only, i.e.

$$\begin{aligned} I_{\mathrm{O}}(\omega) &= \int_{-\infty}^{\infty} dt\, \mathrm{e}^{-i\omega t} \;\; \langle \boldsymbol{u}_i(0)\boldsymbol{u}_i(t)\rangle_{i\in\mathrm{O}} \ , \\ I_{\mathrm{H}}(\omega) &= \int_{-\infty}^{\infty} dt\, \mathrm{e}^{-i\omega t} \;\; \langle \boldsymbol{u}_i(0)\boldsymbol{u}_i(t)\rangle_{i\in\mathrm{H}} \ . \end{aligned} \tag{S6}$$

In the main text this VDOS decomposition into O and H atomic contributions is shown only as an inset in Fig. 3. Here, we again depict these partial VDOS data, this time as a full-sized plot in Fig. S4 for easier visual distinction of the intertwined VDOS intensity curves that quantify single-particle motion. For an analysis of the *correlated* atomic motion in real space, the radially-resolved generalized VDOS concept as defined in Sec. IV F of this Supplemental Material (see Eq. S36) is particularly useful.

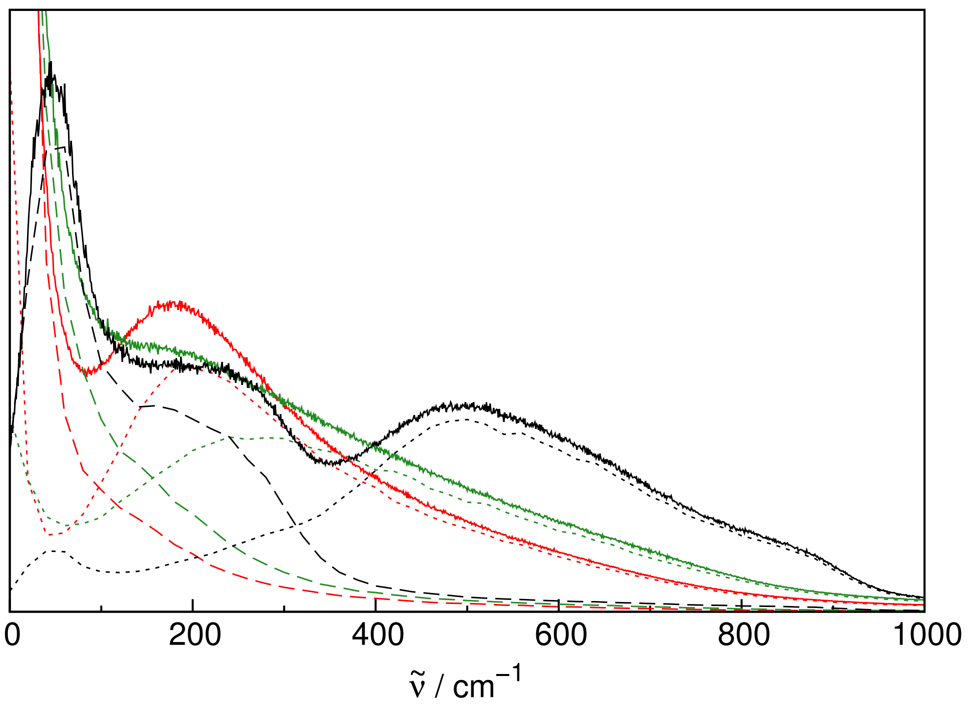


Figure S4. Vibrational density of states with separate contributions due to O (dashed lines) and H (dotted lines) atoms for LD–SCW (red), HD–SCW (green), and RTW (black). The zero-frequency peak of LD– and HD–SCW is off scale.

## IV. COMPUTING INFRARED SPECTRA

### A. Basic Formalism

Linear infrared (IR) spectra at temperature $T$ ($\beta = 1/k_\mathrm{B}T$) are given by the frequency-dependent absorption coefficient $\alpha_\mathrm{IR}$ that is obtained within first-order perturbation (or linear response) theory in terms of the Fourier transform of the autocorrelation function of the total dipole operator $\hat{\boldsymbol{M}}$ of the entire system of volume $V$ and index of refraction $n(\omega)$,

$$\alpha_\mathrm{IR}(\omega) = \frac{4\pi\omega\tanh(\beta\hbar\omega/2)}{3\hbar n(\omega)cV} \int_{-\infty}^{\infty} dt \exp(-i\omega t)\ \frac{1}{2}\,\langle \hat{\boldsymbol{M}}(0)\cdot\hat{\boldsymbol{M}}(t) + \hat{\boldsymbol{M}}(t)\cdot\hat{\boldsymbol{M}}(0)\rangle, \tag{S7}$$

where $c$ is the speed of light. In the classical limit the so-called harmonic approximation,

$$\alpha_\mathrm{IR}(\omega) = \frac{2\pi\omega^2\beta}{3n(\omega)cV} \int_{-\infty}^{\infty} dt \exp(-i\omega t)\ \langle \boldsymbol{M}(0)\cdot\boldsymbol{M}(t)\rangle \tag{S8}$$

$$\equiv \frac{2\pi\beta}{3n(\omega)cV} \int_{-\infty}^{\infty} dt \exp(-i\omega t)\ \langle \dot{\boldsymbol{M}}(0)\cdot\dot{\boldsymbol{M}}(t)\rangle\,, \tag{S9}$$

is used in the following; see Refs. 8–10 for detailed discussions of its merits and note that $1/4\pi\epsilon_0$ factors might be included depending on units. Here, the time-dependent total dipole moment of the sample $\boldsymbol{M}(t)$, or correspondingly its velocity $\dot{\boldsymbol{M}}(t)$, is generated by micro-canonical molecular dynamics simulations using classical nuclei, whereas the thermal average $\langle\ldots\rangle$ must be computed in the canonical ensemble at temperature $T$. The dipole moment can be computed either directly from electronic structure calculations, for instance in the framework of ab initio molecular dynamics [9, 10] or alternatively from parameterized force fields. In the present study, a computationally efficient standard non-polarizable force field for water, namely the flexible SPC model [1], is used to simulate the IR spectra of super-critical water based on using the dipole velocity autocorrelation function.

### B. Torii Corrections for Rigid Non–Polarizable Force Fields

While intermolecular H–bond motion leads to a pronounced peak in the THz region of IR spectra at around 200 cm$^{-1}$ (6 THz) which is reproduced for the right reason by ab initio molecular dynamics simulations [11, 12], this so-called network mode is completely absent when using non-polarizable force fields. Torii developed in 2011 and 2014 two methods, which we call Torii–I [13] and Torii–II [14] schemes for short, to take into account the underlying

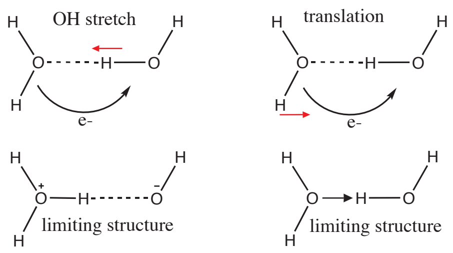


Figure S5. Schematic concept of the charge flux induced by intramolecular vibration (left) and intermolecular translation (right) according to Ref. 13.

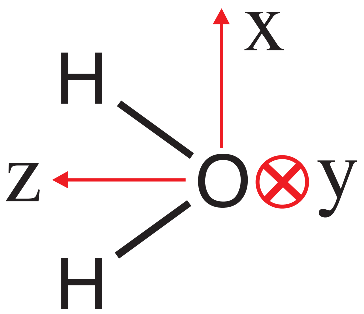


Figure S6. Principal axes system of a water molecule.

intermolecular polarization effects due to H-bond vibrations via adding partial charge fluxes in the framework of simulations based on non-polarizable force fields.

In the Torii–I scheme [13], the total dipole moment velocity of the water system is modified as follows. The total dipole moment is initially split into molecular contributions, $\boldsymbol{M} = \sum \boldsymbol{\mu}(\boldsymbol{r}^{\text{trans}}, \boldsymbol{r}^{\text{rot}}, \boldsymbol{r}^{\text{vib}})$, that depend on translational, vibrational and rotational molecular degrees of freedom so that the total time derivative can be written as

$$\dot{\boldsymbol{M}} = \sum_{\text{molecules}} \left( \frac{\partial \boldsymbol{\mu}}{\partial \boldsymbol{r}^{\text{trans}}} \cdot \dot{\boldsymbol{r}}^{\text{trans}} + \frac{\partial \boldsymbol{\mu}}{\partial \boldsymbol{r}^{\text{rot}}} \cdot \dot{\boldsymbol{r}}^{\text{rot}} + \frac{\partial \boldsymbol{\mu}}{\partial \boldsymbol{r}^{\text{vib}}} \cdot \dot{\boldsymbol{r}}^{\text{vib}} \right) , \tag{S10}$$

where the vibrational part vanishes when a rigid water model is used as in the original study by Torii.

Upon investigating electron density derivatives within finite water clusters using electronic structure (DFT) calculations, intermolecular translation is seen to result in a flux of electrons from an H-bond acceptor molecule to its donor molecule. This is similar, but less pronounced in magnitude, to what happens upon stretching an intramolecular OH-bond as illustrated schematically in Fig. S5. These intermolecular charge fluxes as a result of relative translation of two H-bonded water molecules increase the dipole moment time derivatives and thus result in modified IR intensities. In addition to translation, the rotation of a water molecule results in a reduced effective dipole moment only for rotational motion, $\mu_{\text{eff}}^{\text{rot}}$, compared to the normal dipole moment according to the underlying force field. To correct for this effect, the latter should therefore be scaled accordingly (only) when computing the librational part of the

IR spectrum. Using the molecule-fixed reference frame of Fig. S6, Torii parameterized the four terms compiled in Table II that need to be taken into account to correct the IR spectrum of condensed phase water at frequencies of the librational band and below, thus including the THz regime, when rigid non-polarizable water models are used in molecular dynamics simulations. In the Torii–II scheme [14], the effects of H-bond fluctuations are considered

Table II. Correction terms according to the Torii–I scheme [13] defined with the coordinate system of Fig. S6.

| $v_x = \frac{\partial\mu_x}{\partial r_x^{\mathrm{trans}}}$ | $v_y = \frac{\partial\mu_y}{\partial r_y^{\mathrm{trans}}}$ | $v_z = \frac{\partial\mu_z}{\partial r_z^{\mathrm{trans}}}$ | $\mu_{\mathrm{eff}}^{\mathrm{rot}}$ |
|---|---|---|---|
| 1.91 D Å$^{-1}$ | -1.76 D Å$^{-1}$ | 0 D Å$^{-1}$ | 1.57 D |

by analyzing the derivatives of the electron population with respect to small displacements of tetrahedrally coordinated water molecules in the finite water clusters. These effects are not included in the Torii–I approach [13], because a common set of parameters is used for all molecules therein, independently from their local environment. Based again on electronic structure calculations of water clusters, Torii found that the intermolecular H-bond length, $r_{\mathrm{O\cdots H}}$, is approximately linear w.r.t. the derivative of the magnitude of inter-molecular charge flux (ICF) through this H-bond, i.e.

$$\frac{\partial q^{\mathrm{ICF}}}{\partial r_{\mathrm{O\cdots H}}} = -b_{\mathrm{ICF}}\left(r_{\mathrm{O\cdots H}} - r_{\mathrm{cut}}\right) \qquad \text{where} \qquad r_{\mathrm{O\cdots H}} \leq r_{\mathrm{cut}}\,, \tag{S11}$$

where $q^{\mathrm{ICF}}$ denotes the amount of charge that is transferred from the H-bond acceptor to its donor partner and $b_{\mathrm{ICF}}$ and $r_{\mathrm{cut}}$ are two linear fitting parameters. The distance $r_{\mathrm{cut}}$ is a cutoff for the H-bond length beyond which electron charge is no longer transferred between two water molecules. It is noted in passing that, therefore, this Ansatz does take into account different numbers of H-bonded neighbors around a reference molecule and thus considers topological defects in the H-bond network within the limitations of the aforedescribed parameterization based on electron population analyses. Integration results in an equation for the transferred charge in direct relation to the length of the H-bond

$$q^{\mathrm{ICF}} = \frac{b_{\mathrm{ICF}}}{2}\left(r_{\mathrm{O\cdots H}} - r_{\mathrm{cut}}\right)^2\,. \tag{S12}$$

This allows one to calculate a dipole moment resulting from the ICF simply by determining all H-bond lengths within the system.

Another important mechanism that influences the IR intensity depending on H-bonding is intramolecular polarization of the partial charges of the water molecules by the local electric field due to the surrounding charges. This is obviously not included in non-polarizable water models, but can be incorporated by computing the electric field and using the molecular polarizability tensor $\alpha$ (again computed from DFT calculations and assuming isotropy) that gives rise to an additional dipole moment. The set of parameters for the Torii–II approach [14] is summarized in Table III.

Table III. Correction terms according to the Torii–II scheme [14] defined with the coordinate system of Fig. S6.

| $b_{\mathrm{ICF}}$ | $r_{\mathrm{cut}}$ | $\alpha$ |
|---|---|---|
| 0.0884 $e$ Å$^{-2}$ | 2.374 Å | 1.16 Å$^3$ |

Finally we note that Torii used the identical prefactor in front of the classical dipole autocorrelation function as that of the time symmetrized quantum expression, Eq. (S7), such that a trivial frequency-dependent scaling factor,

$$f(\omega) = \frac{\tanh(\beta\hbar\omega/2)}{\beta\hbar\omega/2}\,, \tag{S13}$$

must be applied when comparing to our results, which are always based on using Eq. (S8), or equivalently Eq. (S9), for multiple reasons that are worked out in Ref. 8.

### C. Torii–I Correction for Flexible Water Models

When using a flexible non-polarizable water model as done in the present simulations, a procedure has to be devised in order to generalize Torii's scheme beyond rigid molecules. Thus, translational, rotational and vibrational motion has to be separated approximately under the assumption that the intramolecular degrees of freedom, i.e. the vibrations, are not affected by the correction which acts exclusively on the former two intermolecular degrees of freedom. Within each molecular dynamics configuration used for analyses each water molecule of the system was analyzed separately by first transforming to center of mass (CM) coordinates and velocities of this molecule,

$$\boldsymbol{R}^{\mathrm{CM}} = \frac{1}{M_{\mathrm{tot}}}\sum_{i=1}^{n} m_i \cdot \boldsymbol{r}_i \quad \text{and} \quad \dot{\boldsymbol{R}}^{\mathrm{CM}} = \frac{1}{M_{\mathrm{tot}}}\sum_{i=1}^{n} m_i \cdot \dot{\boldsymbol{r}}_i\,. \tag{S14}$$

After calculation of the velocities and positions of each atom of this molecule with respect to its CM,

$$\boldsymbol{r}_i^{\mathrm{CM}} = \boldsymbol{r}_i - \boldsymbol{R}^{\mathrm{CM}} \quad \text{and} \quad \dot{\boldsymbol{r}}_i^{\mathrm{CM}} = \dot{\boldsymbol{r}}_i - \dot{\boldsymbol{R}}^{\mathrm{CM}}\,, \tag{S15}$$

the separation would be complete for a rigid water model, since only rotation remains in this case. For flexible models as used in this study, however, $\boldsymbol{r}_i^{\mathrm{CM}}$ combines vibration and rotation. Therefore, the angular velocity $\boldsymbol{\omega}$ of the respective molecule was determined from its instantaneous moment of inertia tensor $\underline{\underline{I}}$ as well as its angular momentum $\boldsymbol{L}$ vector,

$$\boldsymbol{L} = \sum_{i=1}^{n} m_i \boldsymbol{r}_i^{\mathrm{CM}} \times \dot{\boldsymbol{r}}_i^{\mathrm{CM}} = \underline{\underline{I}} \cdot \boldsymbol{\omega} = \left( \sum_{i=1}^{n} m_i \cdot \left( |\boldsymbol{r}_i^{\mathrm{CM}}|^2 \cdot \underline{\underline{1}} - \boldsymbol{r}_i^{\mathrm{CM}} \cdot (\boldsymbol{r}_i^{\mathrm{CM}})^{\mathrm{T}} \right) \right) \cdot \boldsymbol{\omega}\,. \tag{S16}$$

The rotating velocity of each atom $i$ results then from the cross product of angular velocity and the position of the respective atom in CM coordinates. The vibrating velocities remain defined as the difference of the velocity in CM coordinates and the rotating velocity,

$$\dot{\boldsymbol{r}}_i^{\mathrm{rot}} = \boldsymbol{\omega} \times \boldsymbol{r}_i^{\mathrm{CM}}\,, \tag{S17}$$

$$\dot{\boldsymbol{r}}_i^{\mathrm{vib}} = \dot{\boldsymbol{r}}_i^{\mathrm{CM}} - \dot{\boldsymbol{r}}_i^{\mathrm{rot}}\,. \tag{S18}$$

Consequently, the vibrational and rotational (called librational from now on) dipole velocities $\dot{\boldsymbol{\mu}}$ were calculated from the charges $q$ and from the vibrating and rotating velocities, respectively. To Torii-correct the rotational motion, the librational dipole velocities were reduced by the ratio of the effective dipole moment established by Torii, $\mu_{\mathrm{eff}}^{\mathrm{rot}}$, and the dipole moment of the respective water model used, i.e., $\gamma = 1.57\ \mathrm{D}/\mu_{\mathrm{model}}$,

$$\dot{\boldsymbol{\mu}}^{\mathrm{vib/rot}} = \gamma \cdot \sum_{i=1}^{n} q_i \cdot \dot{\boldsymbol{r}}_i^{\mathrm{vib/rot}}\,, \tag{S19}$$

while the dipole vibrations were not corrected, i.e. $\gamma = 1$ in this case, in the spirit of Torii's original rigid-molecule scheme. Since the translational dipole velocity is corrected separately with respect to the principal axes of the water molecule, the axes were determined by diagonalizing the moment of inertia which was already calculated to determine the angular velocity via

$$\underline{\underline{I}} \cdot \boldsymbol{u} = \lambda \cdot \boldsymbol{u} \qquad ; \qquad |\boldsymbol{u}| = 1\,. \tag{S20}$$

Subsequently, the translational dipole velocity follows from the correction of the $\boldsymbol{u}_x$– and $\boldsymbol{u}_y$–axes according to Torii's translational dipole derivatives $v_x$ and $v_y$ as described before,

$$\dot{\boldsymbol{\mu}}^{\mathrm{trans}} = \boldsymbol{u}_x \cdot (\boldsymbol{u}_x \dot{\boldsymbol{R}}^{\mathrm{CM}} v_x) + \boldsymbol{u}_y \cdot (\boldsymbol{u}_y \dot{\boldsymbol{R}}^{\mathrm{CM}} v_y) \quad \text{since } v_z = 0. \tag{S21}$$

The total dipole velocity of the molecule results then from adding the partial velocities, whereas the total dipole velocity per configuration is calculated by summing over the dipole velocities of all molecules in the system,

$$\dot{\boldsymbol{\mu}}^{\text{tot}} = \dot{\boldsymbol{\mu}}^{\text{trans}} + \dot{\boldsymbol{\mu}}^{\text{rot}} + \dot{\boldsymbol{\mu}}^{\text{vib}}\,, \tag{S22}$$

$$\dot{\boldsymbol{M}} = \sum_{\text{molecules}} \dot{\boldsymbol{\mu}}^{\text{tot}}. \tag{S23}$$

The time sequence of total dipole velocities $\dot{\boldsymbol{M}}$ are then correlated and Fourier-transformed according to Eq. (S9) to yield the reported Torii–I corrected IR spectra.

### D. Torii–II Correction for Flexible Water Models

When computing the Torii–II correction, which is based on the dipole moment itself, the librational and vibrational contributions of the molecular dipole moment were calculated from the CM coordinates

$$\boldsymbol{\mu}^{\text{rot+vib}} = \sum_{i=1}^{n} q_i \cdot \boldsymbol{r}_i^{\text{CM}}\,, \tag{S24}$$

which is just the regular dipole moment of the water model. In this case no further separation was necessary since no change of the librational part is envisaged for Torii's second correction. The transferred charge was computed straightforwardly from Eq. (S12) and placed on the oxygen atoms of the involved water molecules, thus yielding the ICF dipole moment per H-bond,

$$\boldsymbol{\mu}^{\text{ICF}} = q^{\text{ICF}} \cdot \left(\boldsymbol{r}_{\text{O,donor}} - \boldsymbol{r}_{\text{O,acceptor}}\right)\,. \tag{S25}$$

The additional intramolecular polarization effects are included by applying the isotropic molecular polarizability $\alpha$ to the electric field $\boldsymbol{E}$ at each molecular CM, $\boldsymbol{R}^{\text{CM}}$. The electric field is calculated following Torii's original procedure (H. Torii, private communication) from all $N-1$ surrounding molecules of the simulation box within the minimum image convention,

$$\boldsymbol{E} = \sum_{i=1,j=1}^{n,N-1} q_{i,j} \frac{\boldsymbol{R}^{\text{CM}} - \boldsymbol{r}_{i,j}}{|\boldsymbol{R}^{\text{CM}} - \boldsymbol{r}_{i,j}|^3}\,, \tag{S26}$$

which yields the resulting dipole moment via

$$\boldsymbol{\mu}^{\text{pol}} = \alpha \boldsymbol{E}\,. \tag{S27}$$

Again, the total dipole moment of the entire configuration results from addition of all partial dipoles,

$$\boldsymbol{M} = \sum_{\text{molecules}} \left(\boldsymbol{\mu}^{\text{rot+vib}} + \boldsymbol{\mu}^{\text{pol}}\right) + \sum_{\text{H-bonds}} \boldsymbol{\mu}^{\text{ICF}}. \tag{S28}$$

The time-evolving total dipole moments $\boldsymbol{M}(t)$ are autocorrelated and Fourier-transformed to yield the reported Torii–II corrected IR spectra according to Eq. (S8).

### E. Torii-Corrected IR Spectra of Supercritical Water

Before applying the two correction schemes to supercritical water obtained from the flexible SPC model, we applied our implementations to TIP4P and TIP5P simulations of water at ambient conditions and compared our results to Torii's published data (we are particularly grateful to H. Torii for detailed explanations as to how his simulations have been carried out, which we reproduced as closely as possible for the sake of one–to–one comparisons). Our data were found to agree closely with the published data when using both the Torii–I [13] and Torii–II [14] schemes. However, it must be noted that the sign of the cross-correlation term of the Torii–I correction as used for the published TIP4P water data (depicted in Fig. 5 of Ref. 13 and again in Fig. 4c of Ref. 14) must be reverted (H. Torii, private communication) as a consequence of using the other sign of the translational dipole derivatives when generating the published TIP4P data. When we use the correct sign, our resulting Torii–I corrected TIP4P spectrum is found to be consistent with the published TIP5P spectrum and shows a much more pronounced translational peak.

Subsequently, both schemes to correct for the neglected polarization effects in non-polarizable force fields were applied to the simulations of the flexible SPC water model [1] in the supercritical regime (at 660 K using densities of 0.2 and 0.6 g/cm$^3$) as well as at ambient conditions for reference (using the same set of trajectories as in the main text). The corresponding spectra of the relevant intermolecular region up to 1100 cm$^{-1}$ are presented in Fig. S7. At ambient conditions both corrections nicely incorporate the desired intermolecular H-bond network peak at around 200 cm$^{-1}$ (6 THz) according to Torii–I [13] and Torii–II [14] schemes. The first correction procedure is seen to reduce the libration intensity too strongly relative to the uncorrected spectrum, but its lineshape is very close to that obtained from the Torii–II correction after scaling up its intensity (cf. panel a to b in Fig. S7).

In stark contrast to water at ambient conditions, where the librational band and the

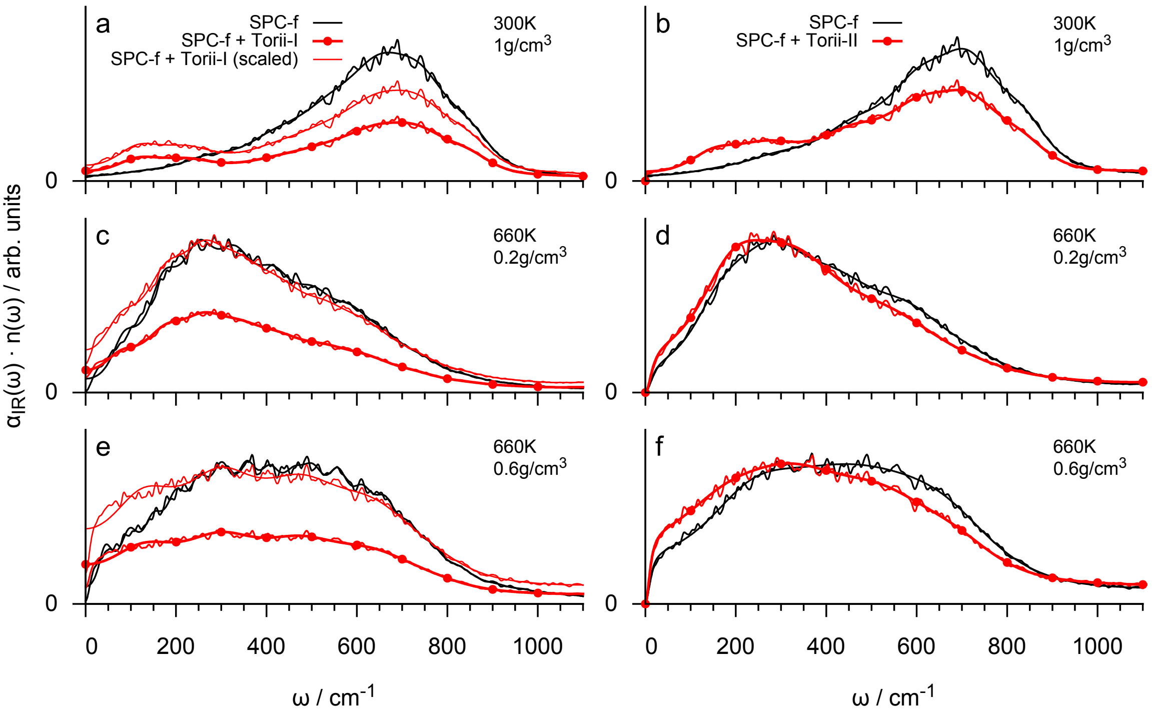


Figure S7. Torii–I (left panels) and Torii–II (right panels) corrected IR spectra obtained from using the flexible SPC model for ambient water (top panels) and supercritical water at 0.2 and 0.6 g/cm$^3$ (center and bottom panels, respectively) and 660 K; the uncorrected reference spectra are shown using black lines. The smooth and noisy spectra were obtained from maximum entropy (red lines with dots) and smoothened Fourier transform (red lines) methods, respectively. The Torii–I spectra have also been scaled up (thin red lines without dots) to reveal better their lineshape.

network mode peak at distinctly different center frequencies, both corrections do not result in significant changes of the IR spectrum in the supercritical regime as obtained from the non-polarizable SPC water model. The IR spectra of supercritical water at the two investigated densities are found to be particularly broad, structureless, and shifted to much lower center frequencies as a result of increasing the temperature and decreasing the density of the fluid (see main text for discussion). Again, the Torii–I correction seems to grossly underestimate the spectral density due to the significant scaling of the molecular dipole moment of the water molecules. Yet, this polarization correction does not affect much the overall shape of the lineshape function in the relevant frequency range, except for increasing the spectral density below roughly 100 and 200 cm$^{-1}$ at the lower and higher density, respectively. The

Torii–II scheme, which does not assume a particular H-bonding pattern and also explicitly includes molecular polarizability depending on the particular molecular configuration of the entire water sample (within the minimum image convention), leads to similarly small changes of the bare SPC reference spectrum. In particular, also the refined Torii–II correction does not affect the overall lineshape of water at supercritical conditions, in stark contrast to its effect on the IR spectrum of water at ambient conditions and thus normal density.

Last but not least, we compare for supercritical water the computed THz spectra in Fig. S7 with and without Torii corrections [13, 14] to published data. These spectra qualitatively agree with limited AIMD simulations of supercritical water at similar state points using the BLYP functional (see Fig. 9 in Ref. 15 and Fig. 11 in Ref. 16) and the BLYP+D3 functional (see Fig. 11 in Ref. 16); note that the agreement is well within the deviations between the two distinct BLYP AIMD spectra that have been published by different groups. Similar accord is reached with reference to the low-frequency IR spectra obtained using the (non–polarizable and uncorrected) SPC/E force field (see inset in bottom panel of Fig. 1 in Ref. 17) and the polarizable so-called TAB/10D force field (see Fig. 5 in in Ref. 18).

Based on this detailed assessment of the two Torii corrections in conjunction with comparison of our spectra to published data, our conclusion is to not apply any such correction to supercritical water when spatially decomposing its IR response or computing the generalized VDOS (as explained in the next Sec. IV F), which are the data presented in the main text in Fig. 4.

### F. Spatially Decomposed Spectral Analysis in Real Space

The intra- and intermolecular correlations underlying the macroscopic IR spectra and the VDOS can be resolved when applying the spatial decomposition scheme, as outlined before for bulk liquid water at ambient conditions [11, 12]. To this end, either molecular dipole velocities $\dot{\boldsymbol{\mu}}_I(t)$ or atomic mass-weighted velocities $\boldsymbol{u}_i(t)$ are projected onto a regular cubic grid $\boldsymbol{r}$ using a Gaussian kernel with a standard deviation $\sigma$ to ensure smooth decomposition,

$$\boldsymbol{j}(t,\boldsymbol{r}) = \sum_{I=1}^{N} \dot{\boldsymbol{\mu}}_I(t) \frac{1}{(2\pi\sigma^2)^{3/2}} \exp\left[-\frac{(\boldsymbol{R}_I(t)-\boldsymbol{r})^2}{2\sigma^2}\right], \tag{S29}$$

$$\boldsymbol{\rho}(t,\boldsymbol{r}) = \sum_{i=1}^{N_{\mathrm{at}}} \boldsymbol{u}_i(t) \frac{1}{(2\pi\sigma^2)^{3/2}} \exp\left[-\frac{(\boldsymbol{r}_i(t)-\boldsymbol{r})^2}{2\sigma^2}\right]. \tag{S30}$$

For the dipole moment case, integration over the system's volume yields the total dipole moment velocity of the system,

$$\dot{\boldsymbol{M}}(t) = \int d^3\boldsymbol{r}\, \boldsymbol{j}(t,\boldsymbol{r}), \tag{S31}$$

and the total dipole moment autocorrelation function might be computed as

$$\left\langle \dot{\boldsymbol{M}}(0)\dot{\boldsymbol{M}}(t) \right\rangle = \int d^3\boldsymbol{\Delta r} \left\langle \int d^3\boldsymbol{r}\, \boldsymbol{j}(\tau,\boldsymbol{r})\boldsymbol{j}(\tau+t,\boldsymbol{r}+\boldsymbol{\Delta r}) \right\rangle = \int d^3\boldsymbol{\Delta r}\, C_{jj}(t,\boldsymbol{\Delta r}). \tag{S32}$$

The spatially resolved correlation function $C_{jj}(t,\boldsymbol{\Delta r})$ describes contributions to the total dipole moment velocity from cross-correlations of projected molecular dipoles separated by $\boldsymbol{\Delta r}$, including also autocorrelations for $\boldsymbol{\Delta r}=0$. For a system that is spatially homogeneous on a long time scale the resulting density is isotropic and after angular averaging leaves only scalar (1D) dependence on the radius $r$ instead of the dependence on a 3D vector $\boldsymbol{r}$,

$$C_{jj}(t,\boldsymbol{\Delta r}) = 4\pi r^2\, C_{jj}^{\mathrm{rad}}(t,r), \tag{S33}$$

which allows to calculate the radially resolved IR absorption cross section of the system as

$$\alpha(\omega,r) = F(\omega) \int_{-\infty}^{\infty} dt\, \mathrm{e}^{-i\omega t}\, 4\pi r^2\, C_{jj}^{\mathrm{rad}}(t,r), \tag{S34}$$

where the $F(\omega)$ prefactor contains the universal constants and ensures satisfying the detailed balance condition of the exact quantum correlation function. Here, as previously [11, 12, 19], we use the so-called "harmonic approximation" for this purpose and $F(\omega) = \frac{1}{n(\omega)} \frac{1}{4\pi\epsilon_0} \frac{2\pi\beta\omega^2}{3Vc}$,

where the system has volume $V$, temperature $T = (k_\mathrm{B}\beta)^{-1}$, $c$ is the speed of light, $\epsilon_0$ the electric permittivity of the vacuum, and $n(\omega)$ is the refractive index of the sample.

Using Eq. S34, the total IR absorption cross section of the system is conveniently expressed in terms of contributions from auto- and cross-correlations of molecular dipoles as a function of the spatial distance $r$,

$$\alpha(\omega) = \int_0^\infty dr\, \alpha(\omega, r)\,. \tag{S35}$$

In an analogous manner one can generalize the standard VDOS (see Eq. S5) by including cross-correlations of atomic velocities that describe correlated nuclear motion. Utilizing the density projection of mass-weighted velocities (Eq. S30) we may write in analogy to Eq. S34,

$$I(\omega, r) = \int_{-\infty}^\infty dt\, \mathrm{e}^{-i\omega t}\, 4\pi r^2\, C_{\rho\rho}^{\mathrm{rad}}(t, r)\,, \tag{S36}$$

which defines the radially resolved correlations in vibrational motion. Note that the standard definition of VDOS involves only autocorrelations of atomic velocities at $r = 0$.

## V. THREE-DIMENSIONAL REPRESENTATION OF THE RADIALLY-RESOLVED SPECTRA

In the main text, we present a two-dimensional map of the radially-resolved spectra (see Fig. 4 therein). In Fig. S8 herein, a three-dimensional representation of the same data is included to offer a different view of the building up of the cross-correlations in these spectra.

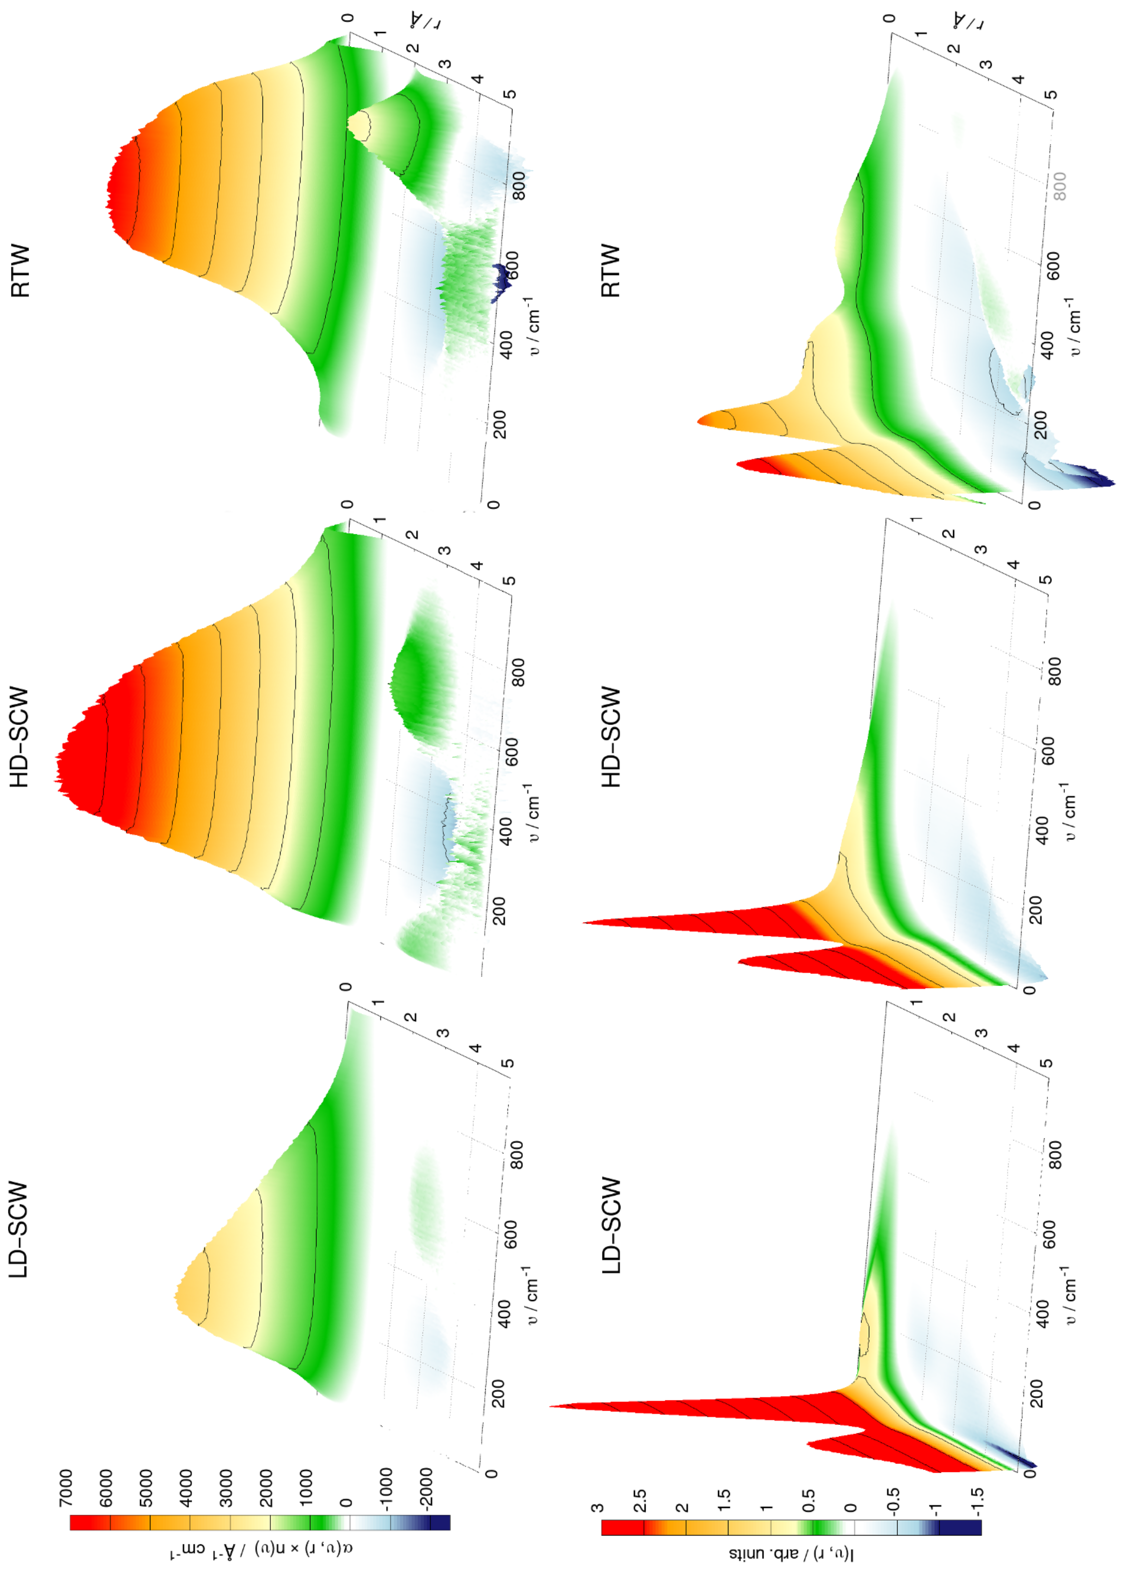


Figure S8. Top: Radially-resolved THz absorption spectra of water at the LD–SCW (left), HD–SCW (middle), and RTW (right) state points. Bottom: Corresponding radially-resolved vibrational correlations (“generalized VDOS”).

### ACKNOWLEDGMENTS

We are particularly grateful to Hajime Torii for his help in communicating the details of the molecular dynamics simulations as well as the computation of the spectra which underlie his publications on the two correction schemes from 2011 and 2014.

[1] K. Toukan and A. Rahman, Phys. Rev. B **31**, 2643 (1985).

[2] A. P. Lyubartsev and A. Laaksonen, Comp. Phys. Commun. **128**, 565 (2000).

[3] G. Raabe and R. J. Sadus, J. Chem. Phys. **126**, 044701 (2007).

[4] A. Luzar and D. Chandler, Phys. Rev. Lett. **76**, 928 (1996).

[5] R. Kumar, J. R. Schmidt, and J. L. Skinner, J. Chem. Phys. **126**, 204107 (2007).

[6] M.-C. Bellissent-Funel, T. Tassaing, H. Zhao, D. Beysens, B. Guillot, and Y. Guissani, J. Chem. Phys. **107**, 2942 (1997).

[7] M. Bernabei, A. Botti, F. Bruni, M.-A. Ricci, and A. K. Soper, Phys. Rev. E **78**, 021505 (2008).

[8] R. Ramírez, T. López-Ciudad, P. Kumar, and D. Marx, J. Chem. Phys. **121**, 3973 (2004).

[9] D. Marx and J. Hutter, *Ab Initio Molecular Dynamics* (Cambridge University Press, Cambridge, 2009).

[10] S. D. Ivanov, A. Witt, and D. Marx, Phys. Chem. Chem. Phys. **15**, 10270 (2013).

[11] M. Heyden, J. Sun, S. Funkner, G. Mathias, H. Forbert, M. Havenith, and D. Marx, Proc. Natl. Acad. Sci. U.S.A. **107**, 12068 (2010).

[12] M. Heyden, J. Sun, H. Forbert, G. Mathias, M. Havenith, and D. Marx, J. Phys. Chem. Lett. **3**, 2135 (2012).

[13] H. Torii, J. Phys. Chem. B **115**, 6636 (2011).

[14] H. Torii, J. Chem. Theory Comput. **10**, 1219 (2014).

[15] M. Boero, K. Terakura, T. Ikeshoji, C. C. Liew, and M. Parrinello, J. Chem. Phys. **115**, 2219 (2001).

[16] R. Jonchiere, A. P. Seitsonen, G. Ferlat, A. M. Saitta, and R. Vuilleumier, J. Chem. Phys. **135**, 154503 (2011).

[17] M. S. Skaf and D. Laria, J. Chem. Phys. **113**, 3499 (2000).

[18] B. D. Bursulaya and H. J. Kim, J. Chem. Phys. **110**, 9656 (1999).

[19] M. Śmiechowski, H. Forbert, and D. Marx, J. Chem. Phys. **139**, 014506 (2013).
